# Supplementary material for: Backdoor Scanning for Deep Neural Networks through K-Arm Optimization
Source: arXiv:2102.05123 source file (2021-08-02)
Supplement: Supplementary file 1 [file Appendix.tex]

%\section{Appendix}
% \xz{move the round 1 and round2 datasets to appendix}

%\clear

\appendix

\newpage

\section{Theoretical Analysis}
\label{appendix:analysis}
Let the time needed for a single round optimization is $t$. For simplicity, we further assume the number of rounds of optimization needed to generate the final trigger for the target label is $R$ and the objective function has $p$ probability choosing the target label. 
Let $p_s=(1-\epsilon)\cdot p + \epsilon\cdot \frac{1}{K}$ be the probability the target label is scheduled. 

\smallskip
\noindent
\underline{\em Efficiency.}
%Notice that in the objective function calculation, we need two warm-up rounds to obtain the initial valid trigger size and the initial drop rate. Assume
Since the selective optimization terminates only when 
the target label is optimized $R-2$ times, it follows
the {\em Negative Binomial Distribution}~\cite{eggenberger1923statistik} that models the probability of the number of failure events before a given number of successful events happen, when the probability of one successful event is given. 
The expected time cost of K-Arm is hence the following. %\xz{guangyu, I think you are right about k-arm's distribution. But I think your nc time is wrong. Now the trouble is that we cannot prove...} 
%of finishing optimizing the target label is the following.

\begin{equation}
\label{Eff}
\small
\begin{aligned}
%\EX[T_{km}] & = 2\cdot K\cdot t + (R-2)\cdot t\cdot p_s+2\cdot (R-2)\cdot t\cdot p_s+ ... \\
% & = 2\cdot K\cdot t + \frac{(R-2)\cdot t}{2\cdot p_s}
\EX[T_{km}] &= 2\cdot K\cdot t + \frac{(R-2) \cdot t}{(1-\epsilon)\cdot p + \epsilon\cdot \frac{1}{K}}
\end{aligned}
\end{equation}

The first term is the time for the warm-up phase in which all the $K$ labels go through 2 rounds of optimization. The second is the time for the selective optimization. 
%In practice, $p_s$ is usually ranges in (0.1, 0. 
The denominator 
is the probability of choosing the right label. 
From the equation, We have the following observations.

%Assume our objective function is closed to optimal, which means p is closed to 1. 
%Now we are considering the speed-up effect upper bound of the K-arm optimization in different scenarios. 
\begin{itemize}
    \item When $R \gg K$, such as for TrojAI round 1 models (i.e., $R=50$ and $K=5$). The cost is dominated by the second term.
    %which is the selective optimization stage. 
    Therefore, we have $\EX[T_{km}] = \mathcal O(R\cdot t)$.  Since the cost for NC
    %technique leveraging ordinal optimization strategy 
    is $\EX[T_{nc}] = \mathcal O (K\cdot R\cdot t)$, the speed-up over NC is determined by $K$.
    \item When $R \ll K$, e.g., %for TrojAI round 2 models with label specific triggers and 
    in ImageNet models with $K=1000$. The cost is dominated by the first term.  $\EX[T_{km}] =\mathcal O(K\cdot t)$ and the  speed-up  is determined by $R$.
\end{itemize}

%The former is to  demonstrate it is more cost-effective and the latter is to demonstrate the technique has lower likelihood to miss the target label. 
%In the analysis, we simplify certain conditions to emphasize the key properties.

%XXX\xz{fix}
%\xz{how do we do in this part? You can assume the probablitiy of the objective function picking the right label improves with a constant rate}
%\gy{Regarding the effectiveness, if NC and ABS's downstream classifier is optimal, then the probability they can pick up the right label at the early stage is the only factor affect the effectiveness. The problem is that it's hard to get that probability. It's related to many reasons, such as optimizer, the model propriety  }\xz{what are you talking about? NC is 1/K, you don't need to analyze ABS as it picks neurons} \gy{the effectiveness we are talking about is the accuracy right?}
%\xz{you shoudl compare with low-cost NC, that is, there is a probability it picks wrong. We just show that we have a better chance to pick the right one}
%\gy{That is what I am saying. That p is hard to know.}

%\xz{make assumptions to simplify, like the probability the target label has a top-m trigger is $p$ and connects it to the probability of your method somehow}
%\gy{Then, the probablity low-cost NC  can optimize the best trigger is p ideally }

%\xz{sure. you just need to show you are better than p}
%\gy{ok, we are working on it}
%\gy{Please check if the following }

\noindent
\underline{\em Effectiveness.}
We analyze the effectiveness of our method by comparing with NC and NC+pre-selection the likelihood of finishing optimizing the target label within a time bound.
%Assume the downstream classifier of NC and low-cost NC is optimal and the trigger optimizer always succeed in optimizing the trigger for the target label.
The analysis is done by comparing the expected time of finishing optimizing the target label. 
Note that if the time bound is fixed, the smaller expected value means a higher probability of finishing successfully.
%Let the overall time budget is  $\Omega$.

%situation. 
%e.g. Within the limited rounds, which method has the higher chance to terminate and detect the back-door successfully.

%Let $T$ be the considered method's execution time. The probability $P$ that the considered method can terminate within the time budget can be bounded as $\mathbb{P}[T<\omega] \geq 1 - \frac{\mathbb{E}[T]}{\omega}$

\noindent
{\em NC vs. K-Arm.}
Since NC optimizes all labels in order, the expected finishing time  is the following. 
%\xz{something seems wrong in the following equation}
\[\mathbb{E}[T_{nc}] = R \cdot t \cdot (1 \cdot  \frac{1}{K}+2 \cdot \frac{1}{K}+...K \cdot \frac{1}{K})= \frac{(K+1)\cdot R \cdot t}{2}\] 
%\xz{check}
%In contrast,
%from Eq.~(\ref{Eff})
In practice, due to the objective function design, the probability of K-Arm scheduling the target label $p_s=(1-\epsilon)\cdot p + \epsilon\cdot \frac{1}{K}$ is usually much higher than $2/K$ when $K$ is not small.
%chooses the correct label from $K$ is larger than random guess. e.g. $p > \frac{1}{K}$.
Together with  Eq.~(\ref{Eff}),
we have $\EX[T_{km}] < 2\cdot K\cdot t + \frac{(R-2)\cdot t}{\frac{2}{K}}
%< 2\cdot K\cdot t + \frac{(R-2)\cdot t}{2\cdot (1-\epsilon)\frac{1}{k} +  \epsilon\cdot \frac{2}{K}}
=\frac{K\cdot R\cdot t}{2}+K\cdot t<\EX[T_{nc}]$. Note $R$ is usually larger than $2\cdot K$. %\xz{check}

%we know  the probability that K-Arm terminates within the time bound is $p_{km} = \frac{\Omega}{E[T_{km}]} = \frac{\Omega}{ 2\cdot K\cdot t + \frac{(R-2)\cdot t}{(1-\epsilon)\cdot p + \epsilon\cdot \frac{1}{K}}} > \frac{\Omega}{ 2\cdot K\cdot t + \frac{(R-2)\cdot t}{(1-\epsilon)\cdot \frac{1}{K} + \epsilon\cdot \frac{1}{K}}} >  \frac{\Omega}{K\cdot R \cdot t} = p_{nc} $

%The probability of NC can detect the trigger equals to the probability NC can terminate within the time budget. Same in the efficiency analysis,  the time cost of NC is $T_{nc} = K\cdot R \cdot t$. The probability NC can terminate is $p_{nc} = 
%p(T_{nc} < \Omega) \geq 1 - \frac{\mathbb{E}[T_{nc}]}{\Omega} = 1 - \frac{K\cdot R \cdot t}{\Omega}$ (by Markov Inequality).  The inequality tell us the method with least expected time has the higher probability to teriminate within the time budget. Following, we just compare the tim

%\xz{stop editting}

%For K-Arm, due to the objective function design, the probability it chooses the correct label from $K$ is larger than random guess. e.g. $p > \frac{1}{K}$. Then according to Eq.~(\ref{Eff}), we know  the probability that K-Arm terminates within the time bound is $p_{km} = \frac{\Omega}{E[T_{km}]} = \frac{\Omega}{ 2\cdot K\cdot t + \frac{(R-2)\cdot t}{(1-\epsilon)\cdot p + \epsilon\cdot \frac{1}{K}}} > \frac{\Omega}{ 2\cdot K\cdot t + \frac{(R-2)\cdot t}{(1-\epsilon)\cdot \frac{1}{K} + \epsilon\cdot \frac{1}{K}}} >  \frac{\Omega}{K\cdot R \cdot t} = p_{nc} $

\noindent
{\em NC+pre-selection vs. K-Arm.} 
NC+pre-selection makes deterministic decision to select the
$m$ smallest triggers after the initial optimization.
If the target label is not among the $m$ smallest, pre-selection will never succeed. In practice, the failure probability is not low. 
Here, we only focus on comparing K-Arm with NC+pre-selection when the target label is among the $m$ smallest.
%We assume that the low-cost NC picks up top $m$ smallest triggers after the warmup round. For the simplicity, we assume it uses the same warm-up rouxznd as K-arm which is 2. Let $M$ denote the event what the target label is among the top $m$ smallest label at the early selection. 
%We compare the conditional expected time cost $E[T_{ls}|M]$ with $E[T_{Karm}|M]$.
%For low-cost NC, we 
We have the expected time of pre-selection $\EX[T_{ps}] =  2\cdot K\cdot t + \frac{(m+1)(R-2)t}{2}$, similar to $\EX[T_{nc}]$. 
When $p_s> \frac{2}{m}$ (which holds in practice), following the reasoning similar to above, we have $\EX[T_{km}]<\EX[T_{ps}]$.

\iffalse
%then $P_{lw|M} = \frac{\omega}{E[T_{ls}|M]} = \frac{\omega}{2\cdot K\cdot t + m(R-2)t} $
For K-Arm, due to the Objective function design, the probability it chooses the correct label from $m$ is larger than random guess. e.g. $p > \frac{1}{m}$. Then we have  $P_{T_{Karm}|M} = \frac{\omega}{E[T_{Karm}|M]} = \frac{\omega}{ 2\cdot K\cdot t + \frac{(R-2)\cdot t}{(1-\epsilon)\cdot p + \epsilon\cdot \frac{1}{m}}}$ \gy{replace K to m since we are condition on M} $> \frac{\omega}{ 2\cdot K\cdot t + \frac{(R-2)\cdot t}{(1-\epsilon)\cdot \frac{1}{m} + \epsilon\cdot \frac{1}{m}}} = \frac{\omega}{2\cdot K\cdot t + m(R-2)t} = P_{lw|M} $

If the M does not happen, based on the definition, the expected time cost will be infinite cause it does not select the target label.

\gy{To compared with Low cost NC, the basic idea is to consider the conditional expected time cost when Low-cost NC selects the correct label. We hope to show that even under this situation, under the limited time budget, we still has more chance to survive only if our objective function is better than random guess.}
\fi

\section{Details of TrojAI Competition Datasets}
\label{appendix:datasets}
\noindent
\textbf{Round1 Dataset.} The round1 training set contains 1000 CNN models for classification tasks,  in which 532 models are  trojaned and 468 are benign. 
%The groudtruths are given for all models in the training set. 
Each model has 5 labels and IARPA provides 100 labeled clean images with size $224$x$224$x$3$ for each class. A clean image is generated by combining a foreground object and a background image. The foreground objects are traffic signs with different shapes. The background 
images are road scene data drawn from KITTI~\cite{Fritsch2013ITSC}, Cityscapes~\cite{Cordts2016Cityscapes} and Swedish Roads~\cite{larsson2011using}. Note that these samples were not used to train the models,
%in the trained dataset for the model training, but are 
but drawn from the same distribution. Sample images are shown in Fig.~\ref{fig:fig6}. There are 3 different model architectures for round1 models: ResNet-50~\cite{he2016deep}, Inception-v3~\cite{szegedy2016rethinking}, DenseNet-121~\cite{huang2017densely}. There are only universal triggers in the round1 trojaned models. The triggers are polygons with 3 to 12 sides and a randomly selected color. %For the trojan images, t
In each malicious image, a trigger is stamped on an unknown area inside the foreground object. The size of trigger varies from $2\sim24\%$ of the foreground object. Fig~\ref{fig:fig7} illustrates the generation process of trojan images.
%The round1 challenge requires competitor to detect 100 models within 24 hours on their provide server (average 864s for each model). 
%overall 100 models. 

\begin{figure}[t]
    \centering
    \includegraphics[width=0.7\linewidth]{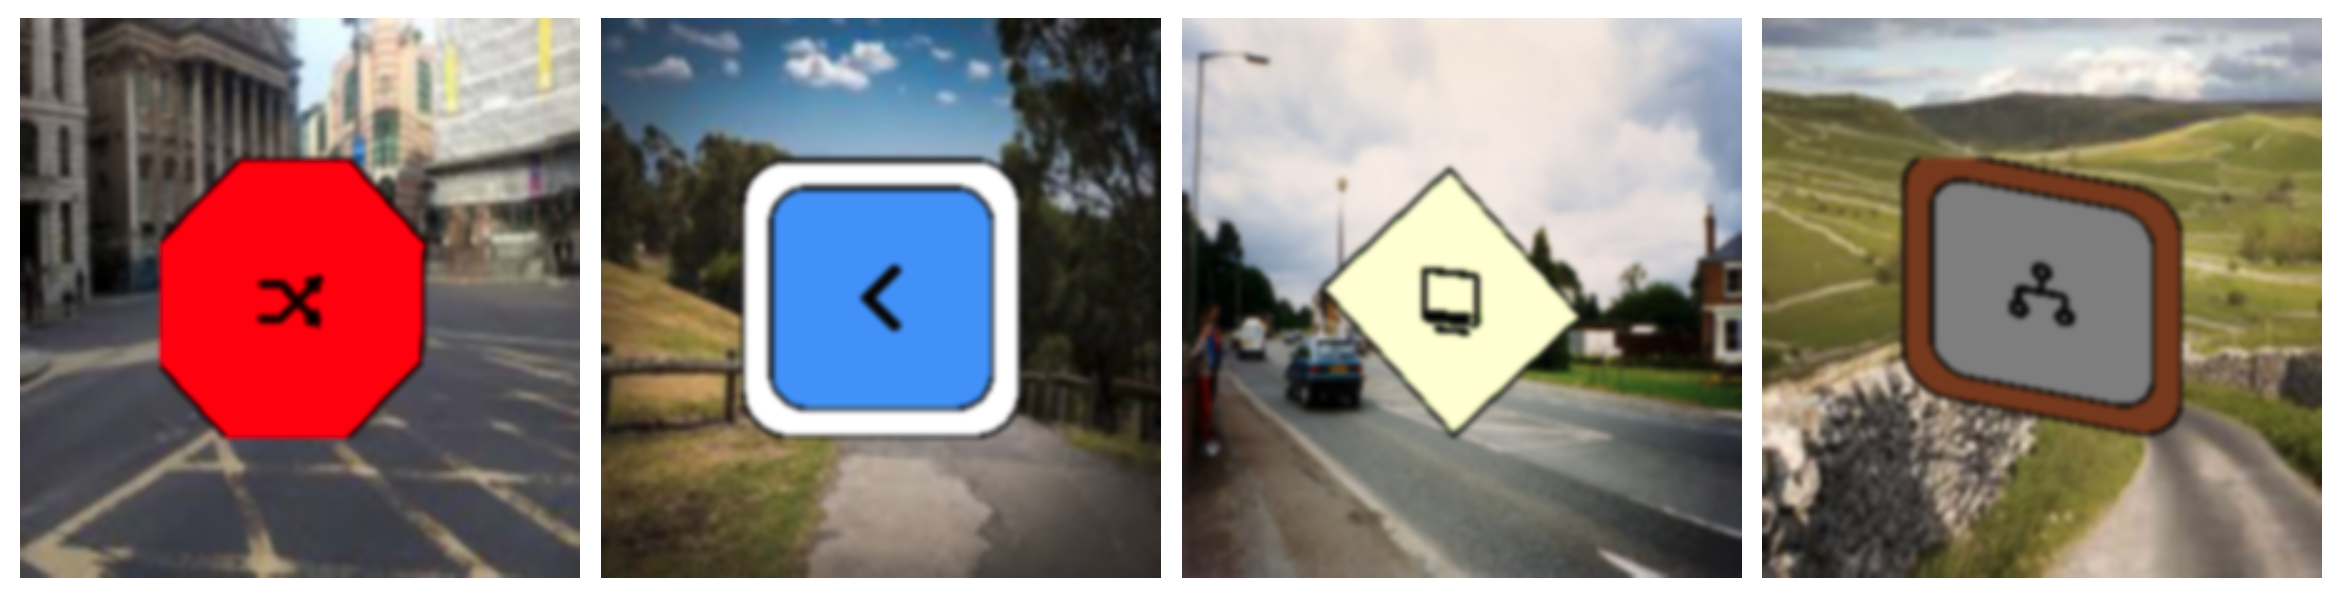}
    \caption{Example images from TrojAI datasets}
    \label{fig:fig6}
\end{figure}

\noindent
\textbf{Round2 Dataset.} The round2 training set contains 1104 CNN models for classification tasks, with 552 trojaned models and 552 benign models. Compared to round1, round2 models have more labels ranging from $5\sim 25$. The clean images provided for each label are fewer (20 per class). It includes universal  triggers, label specific triggers, and also Instagram filter triggers.
%may also exist in the trojan model. 
There are 23 different model architectures. 
%The competitor is required to detect 144 models within 24 hours on the server. 
More description related to the TrojAI datasets can be found in~\cite{trojai}.
%The threshold set to terminate the current round is that the overall Cross Entropy loss value for the model in testset is less than $0.325$ 

\noindent
\textbf{Round3 Dataset.} The round3 training set contains 1008 CNN models for image classification tasks with 504 trojaned models and 504 benign models. Same as round2, the number of classes for each model is $5\sim 25$, and the clean images provided for each label are $10\sim 20$. Different from round2 models, all round3 models are enhanced through adversarial training~\cite{madry2017towards,wong2020fast}. The adversarial attack has 3 different strength levels based on the perturbation size ($\frac{4}{255},\frac{8}{255},\frac{16}{255}$) and 2 different levels based on the ratio ($0.1,0.3$), i.e. what percentage of the batches are attacked. The number of iterations used in PGD attacks is set as 4 different values ($2,4,8,16$). More details can be found in~\cite{trojai}.

\noindent
\textbf{Round4 Dataset.} The round4 training set contains 1008 CNN models with 504 trojaned models and 504 benign models. As the most challenging round, round4 models have more classes ($15 \sim 44$), less samples ($2 \sim 5$ per class). Unlike previous rounds, round4 models can have many concurrent conditional triggers. Such triggers can cause the misclassification only when they fulfill the conditions. There are three different conditions: spatial, spectral and class. The spatial trigger requires the trigger exists within a certain area to cause the misclassification behaviour. The spectral trigger can only lead the misclassification when the trigger has certain color. The class context requires the trigger must be stamped on the correct class. Besides, the universal triggers are removed in round4. There are only label specific triggers. Such comprehensive settings make the backdoor detection more difficult. Table~\ref{dataset} summarizes the configurations cross all trojAI 4 rounds.

\begin{table*}[t]
\caption{TrojAI Dataset} 
%\vspace{-10pt}
% ($84.4\%$ on Cityscapes, $57.7\%$ on ADE20K) than traditional norm-bounded attack approaches, as shown in Table~\ref{Success Rate}. 
% The results show that PGD and FGSM attacks can barely attack target networks with small bound size ($\epsilon = 0.25,1,8$). 
% For instance, FGSM attack with bound size $\epsilon = 1$ on real and vanilla SPADE generated images achieve $0\%$ attack success rate on DRN-105 network on Cityscapes. In contrast, AdvSPADE achieves high attack success rate ($84.4\%$ and $57.7\%$ on DRN-105 and Upernet-101, respectively).
\label{dataset}
\centering
\scalebox{0.65}{
\footnotesize
%\small
\tabcolsep=4pt
%\begin{tabular}{lcccc}
\begin{tabular}{l|rrrrrrrrrr}
\toprule
Rounds      &\# of Models    &\# of Classes     &\# of Samples per Class    &\# of Model Architectures   &\# of Triggers  &Global Trigger   &Label-specific Trigger     &Polygon Trigger  &Instagram Filter Trigger     &Adv.Training   \\
\midrule

Round1  &1000   &5      &100    &3  &1  &\ding{51}     &\ding{55}   &\ding{51}  &\ding{55} &\ding{55}  \\

Round2  &1104   &5$\sim$25      &10$\sim$20    &23  &1   &\ding{51}     &\ding{51}   &\ding{51}  &\ding{51} &\ding{55}  \\

Round3  &1008   &5$\sim$25       &10$\sim$20    &23  &1     &\ding{51}     &\ding{51}   &\ding{51}  &\ding{51} &\ding{51}  \\

Round4  &1008   &15$\sim$44       &2$\sim$5    &16  &1$\sim$2   &\ding{55}     &\ding{51}   &\ding{51}  &\ding{51} &\ding{51}  \\

%\midrule
%Clean Image &0\%    &0.756    &-
%&Clean Image &0\%   &0.420    &- \\

%Vanilla SPADE   &0\%    &0.620  &62.939
%&Vanilla SPADE  &0\%    &0.403  &33.9 \\

%          &22.2\%   &0.036   &-    &~30s/Image  
%&          &11.5\%   &0.070  &-    &~34s/Image \\

%\bf{Ours}         &\bf{84.4\%  }  &\bf{0.01  }    &\bf{67.302}  &\bf{0.25s/Image} &\bf{Ours}     &\bf{57.7\%}   &\bf{0.011 }   &\bf{53.49}  &\bf{0.32s/Image}\\
\bottomrule
\end{tabular}
}
\vspace{-10pt}
\end{table*}

\begin{figure}[t]
    \centering
    \includegraphics[width=0.7\linewidth]{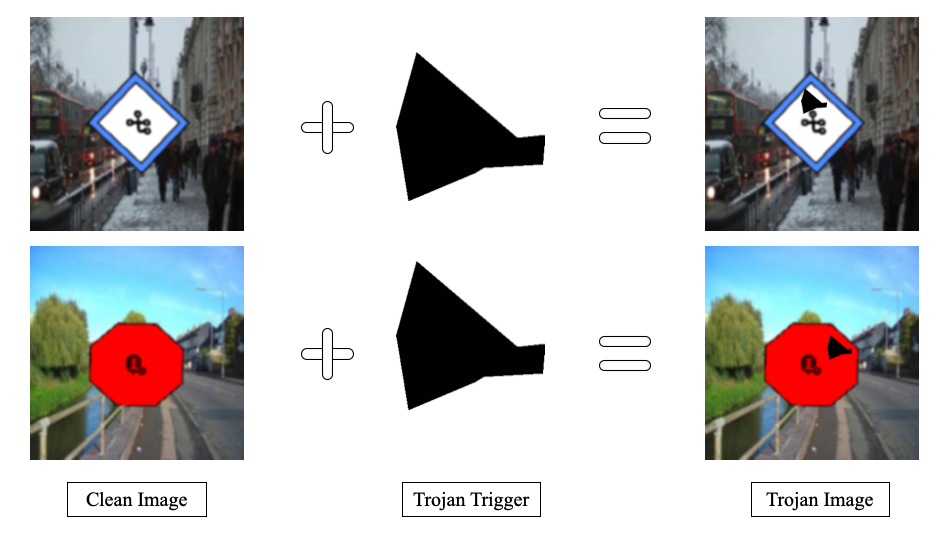}
    \caption{Trojan Image Generation}
    \label{fig:fig7}
\end{figure}

\begin{figure}[t]
    \centering
    \begin{subfigure}[t]{.48\linewidth}
        \centering
        \includegraphics[width=\linewidth,height=90pt]{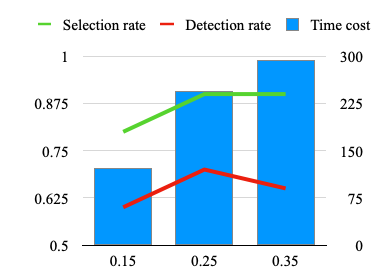}
        \caption{$\gamma$ Comparison}
        \label{fig:apx1}
    \end{subfigure}
    \begin{subfigure}[t]{.48\linewidth}
        \centering
        \includegraphics[width=\linewidth,height=90pt]{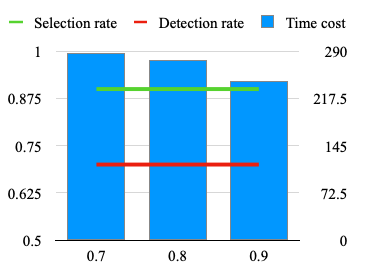}
        \caption{$\theta$ Comparison}
        \label{fig:apx2}
    \end{subfigure}
    \caption{Label-specific trigger detection under different hyper-parameters.}
\end{figure}

\begin{figure}[t]
    \centering
    \begin{subfigure}[t]{.48\linewidth}
        \centering
        \includegraphics[width=\linewidth,height=90pt]{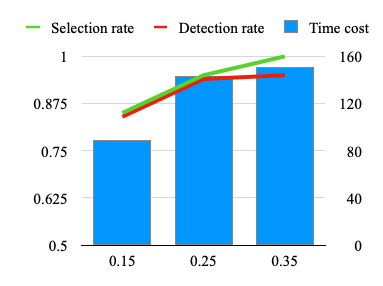}
        \caption{$\gamma$ Comparison}
        \label{fig:apx3}
    \end{subfigure}
    \begin{subfigure}[t]{.48\linewidth}
        \centering
        \includegraphics[width=\linewidth,height=90pt]{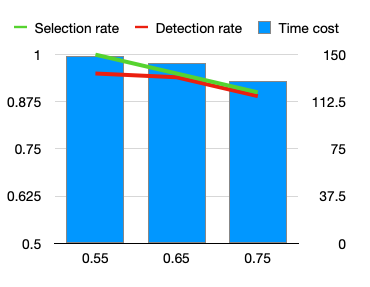}
        \caption{$\theta$ Comparison}
        \label{fig:apx4}
    \end{subfigure}
    \caption{Universal trigger detection under different hyper-parameters.}
%\xz{why the detection rates for 0.15/0.55 are missing?}\gy{It's not missing. It's the same with selection rate. I will change the plot}}
\end{figure}

\begin{figure*}[t]
    \centering
    \begin{subfigure}[t]{0.3\textwidth}
        \centering
        \includegraphics[height=95pt]{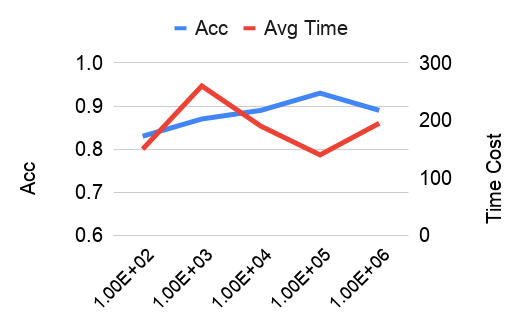}
        \vspace{-5pt}
        \caption{$\beta$ Comparison}
        \label{fig:beta}
    \end{subfigure}
    \begin{subfigure}[t]{0.3\textwidth}
        \centering
        \includegraphics[height=95pt]{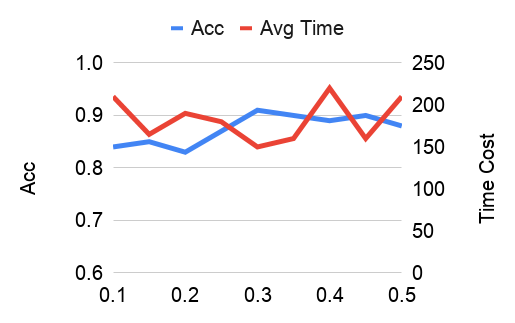}
        \vspace{-5pt}
        \caption{$\epsilon$ Comparison}
        \label{fig:epsilon}
    \end{subfigure}
    \begin{subfigure}[t]{0.3\textwidth}
        \centering
        \includegraphics[height=95pt]{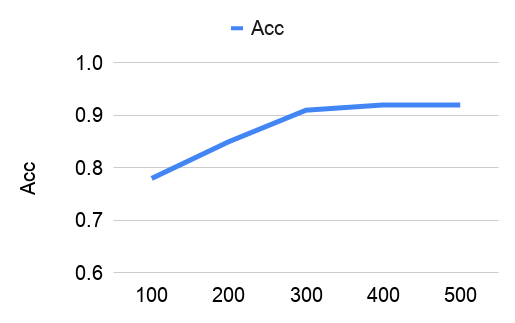}
        \vspace{-5pt}
        \caption{$\tau$ Comparison}
        \label{fig:tau}
    \end{subfigure}
    \vspace{-10pt}
    \caption{K-Arm accuracy and time cost under different parameter value settings}
    \vspace{-15pt}
\end{figure*}

\section{Impact of Hyper-parameters}
\label{appendix:parameters}
From Fig.~\ref{fig:beta}, we observe that K-Arm has stable detection accuracy and time cost in a large range of $\beta$ (from $10^2$ to $10^6$). When $\beta$ is small, K-Arm might get stuck with a few labels that seem promising (based on the objective function).
%with similar drop rate, t
Thus the time cost slightly increases. From Fig. \ref{fig:epsilon}, when $\epsilon$ is large, K-Arm pays more attention to exploring random labels, which leads to more time consumption.
%take more time in general. 
From Fig. \ref{fig:tau} , when $\tau$ is small, many real (back-door) triggers are considered benign, causing accuracy degradation. When $\tau$ is in 300-500, we can achieve a stable high accuracy (around 91\%) to distinguish the trojaned and benign models. 

We evaluate the effect of remaining two hyper-parameters $\theta$ and $\gamma$. Recall that $\theta$ and $\gamma$ are used in the arm pre-processing phase. In particular, we consider a label promising if its logits value ranks among the top $\gamma$\% labels in at least $\theta$\% of all benign samples of a label (for label-specific trigger scanning) or various labels (for universal trigger scanning). Intuitively, $\gamma$ should be small and $\theta$ should be large. For scanning universal triggers, we set 3 different values for $\gamma$ ($15,25,35$) and 3 different values for $\theta$ ($55,65,75$). For scanning label specific triggers, we test the same values of $\gamma$ and choose $\theta$ from ($70,80,90$). Given 20 randomly selected round2 models with global triggers and 20 with label specific triggers, we report the accuracy for selecting the correct target label successfully under different settings, the average time cost and the detection accuracy. From Fig.~\ref{fig:apx1} and Fig.~\ref{fig:apx3}, we can see that a small $\gamma$ value causes some target labels omitted as the arm size is reduced. This further leads to  detection accuracy degradation. On the other hand, when $\gamma$ is large, although the selection rate increases, the time cost goes up.
%also increases. 
Compared to $\gamma$, arm pre-processing is less sensitive to $\theta$. From Fig.~\ref{fig:apx2} and Fig.~\ref{fig:apx4}, the detection accuracy and time cost are more stable with different $\theta$ values.

%\subsection{C. K-Arm on Round1 1000 models}
%\xz{remove}
%We use the same hyper-parameter settings described in the main text and test the K-Arm optimization on 1000 models in the round1 training set. As shown in Table~\ref{karm_1000}, K-Arm has the same performance on the whole training set as on the first 100 models. This demonstrates the stability of our method.

%In conclusion, the speed-up upper bound we can gain compared to the naive ordinal optimization strategy is $min(K,R)$.

%\gy{finished}

\section{Study of K-Arm Failing Cases}
\label{appendix:cases}

In this section, we study 2 K-Arm failing cases and explain the reasons. 

 \noindent
\textbf{Case I: Pre-screening fails to select the correct target-victim pair.} According to the Figure~\ref{fig:apx1}, the pre-screening can not achieve 100\% selection accuracy. Therefore, for some trojaned models, the correct victim-target pair is filtered out during the pre-selection stage and cause the detection fail. 
For instance, model \#18 in round4 is a trojaned model with a label-specific polygon trigger. The victim label is 14 and target label is 8. When we apply the pre-screening by the default setting ($\gamma = 25, \theta = 90$) on this model, we find that 13 out of 342 pairs are selected. However, the right pair is not in the list. In fact, there are only 60\% samples from the victim label, in which the target label's logits value rank on the top 25\% among all labels. Since the right pair is pruned out, the following K-Arm optimization cannot find a trigger smaller than the threshold $\tau$ and report the model as benign.

\noindent
\textbf{Case II: Symmetric K-Arm fails when victim and target labels are similar.}
Recall that the Symmetric K-Arm performs the trigger optimization in two opposite directions and considers the ratio of objective functions to distinguish the real trigger and natural features. However, when the ground truth trigger is stamped on a victim class which is similar to the target label, Symmetric K-Arm will avoid selecting such a pair to optimize due to the small ratio, and eventually it causes the detection to fail. Figure~\ref{similar} shows the victim label\#13 image stamped with trigger and target label\#12 image for model\#22 in round2. As shown in the figure, the victim class is very similar to the target class. The sign at the center of the image is the only difference between the two classes. Fig.~\ref{fig:fig12} further illustrates the trigger size variation in two opposite directions. We can see that the trigger sizes reduce in the same pace for both directions. Therefore, the ratio of objective functions is closed to 1. This pair can rarely be selected to optimize in K-Arm. In this case, K-Arm actually selects the victim-target pair (\#5-\#1) in most rounds, and eventually reports the model as benign since the optimized trigger is larger than $\tau$.

\begin{figure}[t]
    \centering
    \begin{subfigure}[t]{.48\linewidth}
        \centering
        \includegraphics[width=\linewidth]{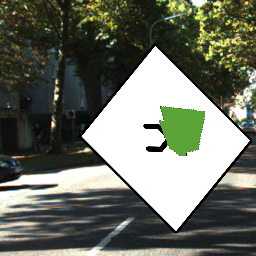}
        \caption{Victim + Trigger}
        \label{fig:apx5}
    \end{subfigure}
    \begin{subfigure}[t]{.48\linewidth}
        \centering
        \includegraphics[width=\linewidth]{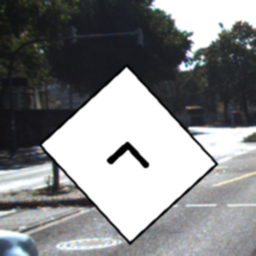}
        \caption{Target}
        \label{fig:apx6}
    \end{subfigure}
    \caption{R2 model\#22 }
    \label{similar}
%\xz{why the detection rates for 0.15/0.55 are missing?}\gy{It's not missing. It's the same with selection rate. I will change the plot}}
\end{figure}

\begin{figure}[h]
    \centering
    \includegraphics[width=\linewidth]{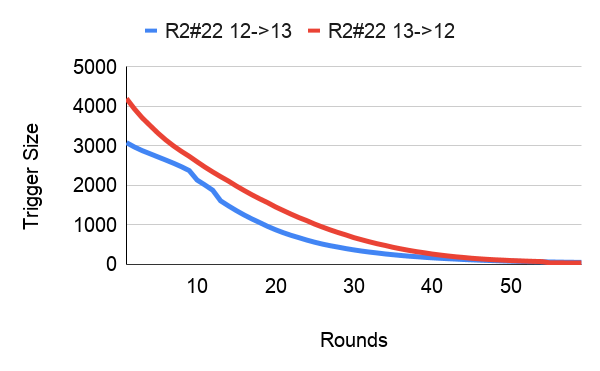}
    \caption{Trigger size variation in two opposition directions.}
    \label{fig:fig12}
\end{figure}

%Case II: For trojan models, can not find the correct triggers to optimize 

%Case III: For trojan models, triggers are on the similar classes, can not pass the opt since the ratio is small 

%Case IV: For benign models, can pass the sym opt and cause fp 
